# Supplementary material for: Search for Cosmic-Ray Electron and Positron Anisotropies with Seven Years of Fermi Large Area Telescope Data
Source: arXiv:1703.01073 ancillary file (2017-03-03)
Supplement: Supplementary file 1 [file LATCREAnis2_SOM_PRLReSub.pdf]

# Supplemental Material: Search for Cosmic-Ray Electron and Positron Anisotropies with Seven Years of Fermi Large Area Telescope Data


S. Abdollahi,[1] M. Ackermann,[2] M. Ajello,[3] A. Albert,[4] W. B. Atwood,[5] L. Baldini,[6,7] G. Barbiellini,[8,9] R. Bellazzini,[7] E. Bissaldi,[10,11] E. D. Bloom,[12] R. Bonino,[13,14] E. Bottacini,[12] T. J. Brandt,[15] P. Bruel,[16] S. Buson,[15] M. Caragiulo,[10,11] E. Cavazzuti,[17] A. Chekhtman,[18] S. Ciprini,[17,19] F. Costanza,[11,*] A. Cuoco,[13,20] S. Cutini,[17,19] F. D'Ammando,[21,22] F. de Palma,[11,23] R. Desiante,[13,24] S. W. Digel,[12] N. Di Lalla,[6,7] M. Di Mauro,[12] L. Di Venere,[10,11] B. Donaggio,[25] P. S. Drell,[12] C. Favuzzi,[10,11] W. B. Focke,[12] Y. Fukazawa,[1] S. Funk,[26] P. Fusco,[10,11] F. Gargano,[11] D. Gasparrini,[17,19] N. Giglietto,[10,11] F. Giordano,[10,11] M. Giroletti,[21] D. Green,[27,15] S. Guiriec,[15] A. K. Harding,[15] T. Jogler,[28] G. Jóhannesson,[29] T. Kamae,[30] M. Kuss,[7] S. Larsson,[31,32] L. Latronico,[13] J. Li,[33] F. Longo,[8,9] F. Loparco,[10,11] P. Lubrano,[19] J. D. Magill,[27] D. Malyshev,[26] A. Manfreda,[6,7] M. N. Mazziotta,[11,†] M. Meehan,[34] P. F. Michelson,[12] W. Mitthumsiri,[35] T. Mizuno,[36] A. A. Moiseev,[27,37] M. E. Monzani,[12] A. Morselli,[38] M. Negro,[13,14] E. Nuss,[39] T. Ohsugi,[36] N. Omodei,[12] D. Paneque,[40] J. S. Perkins,[15] M. Pesce-Rollins,[7] F. Piron,[39] G. Pivato,[7] G. Principe,[26] S. Rainò,[10,11] R. Rando,[25,41] M. Razzano,[7] A. Reimer,[42,12] O. Reimer,[42,12] C. Sgrò,[7] D. Simone,[11] E. J. Siskind,[43] F. Spada,[7] G. Spandre,[7] P. Spinelli,[10,11] A. W. Strong,[44] H. Tajima,[45,12] J. B. Thayer,[12] D. F. Torres,[33,46] E. Troja,[15,27] J. Vandenbroucke,[34] G. Zaharijas,[47,48] and S. Zimmer[49]

(The Fermi-LAT collaboration https://www-glast.stanford.edu/)

[1]*Department of Physical Sciences, Hiroshima University, Higashi-Hiroshima, Hiroshima 739-8526, Japan*
[2]*Deutsches Elektronen Synchrotron DESY, D-15738 Zeuthen, Germany*
[3]*Department of Physics and Astronomy, Clemson University, Kinard Lab of Physics, Clemson, SC 29634-0978, USA*
[4]*Los Alamos National Laboratory, Los Alamos, NM 87545, USA*
[5]*Santa Cruz Institute for Particle Physics, Department of Physics and Department of Astronomy and Astrophysics, University of California at Santa Cruz, Santa Cruz, CA 95064, USA*
[6]*Dipartimento di Fisica "Enrico Fermi" dell'Università di Pisa, I-56126 Pisa, Italy*
[7]*Istituto Nazionale di Fisica Nucleare, Sezione di Pisa, I-56127 Pisa, Italy*
[8]*Istituto Nazionale di Fisica Nucleare, Sezione di Trieste, I-34127 Trieste, Italy*
[9]*Dipartimento di Fisica, Università di Trieste, I-34127 Trieste, Italy*
[10]*Dipartimento di Fisica "M. Merlin" dell'Università e del Politecnico di Bari, I-70126 Bari, Italy*
[11]*Istituto Nazionale di Fisica Nucleare, Sezione di Bari, I-70126 Bari, Italy*
[12]*W. W. Hansen Experimental Physics Laboratory, Kavli Institute for Particle Astrophysics and Cosmology, Department of Physics and SLAC National Accelerator Laboratory, Stanford University, Stanford, CA 94305, USA*
[13]*Istituto Nazionale di Fisica Nucleare, Sezione di Torino, I-10125 Torino, Italy*
[14]*Dipartimento di Fisica, Università degli Studi di Torino, I-10125 Torino, Italy*
[15]*NASA Goddard Space Flight Center, Greenbelt, MD 20771, USA*
[16]*Laboratoire Leprince-Ringuet, École polytechnique, CNRS/IN2P3, F-91128 Palaiseau, France*
[17]*Agenzia Spaziale Italiana (ASI) Science Data Center, I-00133 Roma, Italy*
[18]*College of Science, George Mason University, Fairfax, VA 22030, resident at Naval Research Laboratory,*

*Washington, DC 20375, USA*
[19]*Istituto Nazionale di Fisica Nucleare, Sezione di Perugia, I-06123 Perugia, Italy*
[20]*RWTH Aachen University, Institute for Theoretical Particle Physics and Cosmology, (TTK), D-52056 Aachen, Germany*
[21]*INAF Istituto di Radioastronomia, I-40129 Bologna, Italy*
[22]*Dipartimento di Astronomia, Università di Bologna, I-40127 Bologna, Italy*
[23]*Università Telematica Pegaso, Piazza Trieste e Trento, 48, I-80132 Napoli, Italy*
[24]*Università di Udine, I-33100 Udine, Italy*
[25]*Istituto Nazionale di Fisica Nucleare, Sezione di Padova, I-35131 Padova, Italy*
[26]*Erlangen Centre for Astroparticle Physics, D-91058 Erlangen, Germany*
[27]*Department of Physics and Department of Astronomy, University of Maryland, College Park, MD 20742, USA*
[28]*Friedrich-Alexander-Universität, Erlangen-Nürnberg, Schlossplatz 4, 91054 Erlangen, Germany*
[29]*Science Institute, University of Iceland, IS-107 Reykjavik, Iceland*
[30]*Department of Physics, Graduate School of Science, University of Tokyo, 7-3-1 Hongo, Bunkyo-ku, Tokyo 113-0033, Japan*
[31]*Department of Physics, KTH Royal Institute of Technology, AlbaNova, SE-106 91 Stockholm, Sweden*
[32]*The Oskar Klein Centre for Cosmoparticle Physics, AlbaNova, SE-106 91 Stockholm, Sweden*
[33]*Institute of Space Sciences (IEEC-CSIC), Campus UAB, E-08193 Barcelona, Spain*
[34]*Department of Physics, University of Wisconsin-Madison, Madison, WI 53706, USA*
[35]*Department of Physics, Faculty of Science, Mahidol University, Bangkok 10400, Thailand*
[36]*Hiroshima Astrophysical Science Center, Hiroshima University, Higashi-Hiroshima, Hiroshima 739-8526, Japan*
[37]*Center for Research and Exploration in Space Science and Technology (CRESST) and NASA Goddard Space Flight Center, Greenbelt, MD 20771, USA*
[38]*Istituto Nazionale di Fisica Nucleare, Sezione di Roma "Tor Vergata", I-00133 Roma, Italy*
[39]*Laboratoire Univers et Particules de Montpellier, Université Montpellier, CNRS/IN2P3, F-34095 Montpellier, France*
[40]*Max-Planck-Institut für Physik, D-80805 München, Germany*
[41]*Dipartimento di Fisica e Astronomia "G. Galilei", Università di Padova, I-35131 Padova, Italy*
[42]*Institut für Astro- und Teilchenphysik and Institut für Theoretische Physik, Leopold-Franzens-Universität Innsbruck, A-6020 Innsbruck, Austria*
[43]*NYCB Real-Time Computing Inc., Lattingtown, NY 11560-1025, USA*
[44]*Max-Planck Institut für extraterrestrische Physik, D-85748 Garching, Germany*
[45]*Solar-Terrestrial Environment Laboratory, Nagoya University, Nagoya 464-8601, Japan*
[46]*Institució Catalana de Recerca i Estudis Avançats (ICREA), E-08010 Barcelona, Spain*
[47]*Istituto Nazionale di Fisica Nucleare, Sezione di Trieste, and Università di Trieste, I-34127 Trieste, Italy*

[48]*Laboratory for Astroparticle Physics, University of Nova Gorica, Vipavska 13, SI-5000 Nova Gorica, Slovenia*
[49]*Département de Physique Nucléaire et Corpuscolaire (DPNC), University of Geneva, CH-1211 Genéve 4, Switzerland*
(Dated: March 3, 2017)

We provide additional details on the analysis presented in the main article. These include details on the analysis methods, the procedure used to optimize the event selection and the calculation of the upper limit of the dipole anisotropy.

## CONSTRUCTION OF REFERENCE MAP

We use four methods to create the reference sky map based on the observed data: shuffling technique (Method 1); event rate technique (Method 2); event time sequence randomly chosen from an exponential distribution with given average rate and angles ($\theta$, $\phi$) randomly chosen from real events (Method 3); event time sequence fixed to the observed one and angles ($\theta$, $\phi$) extracted from the real angle distribution (Method 4).

Method 1 by construction preserves exactly the energy and angular distributions (in the LAT reference frame), and also accounts for the detector dead times, since it is based on the instantaneous event rate. However, Method 1 (shuffling) (and Method 4) uses the same event time sequence as the actual data, and this could create some biases in building the reference sky maps, in particular when anisotropies on large angular scales are investigated.

In the above methods the angles ($\theta$, $\phi$) could also be extracted from the Monte Carlo simulated data sample used to build the IRF, which would be equivalent to the exposure method with the Monte Carlo-based acceptance. However, any possible systematic uncertainties arising from the calculation of the instrument acceptance could be large with respect to (w.r.t.) the significance level explored in the analysis [1].

## VALIDATION STUDIES WITH AN IDEAL INSTRUMENT

To check the analysis methods adopted in the current work, we use a simulation with an ideal detector with different FoVs with radii ranging from 40° to 180° and fully efficient within the FoV. In particular we look for any bias in the measured APS and in the white noise value. It is worth pointing out that the knowledge of the white noise allows us to calculate the confidence belt regions for the null hypothesis.

We perform 1000 independent realizations with an isotropic event distribution with a 0.1 Hz rate, covering the same time interval as the current analysis (i.e., 7 years). We perform the simulation including the real spacecraft position, attitude, and livetime time history of the LAT. For each detector we assume a perfect efficiency in the given FoV. We do not include any effects due to the geomagnetic field and Earth shadowing, and this makes the simulation ideal in particular for instruments with very large FoV (> 90°).

The simulated event samples are analyzed with the same chain as for the actual data, by selecting Good Time Intervals (GTIs) when the LAT is operating in standard sky survey mode outside the South Atlantic Anomaly (SAA) and removing the times when the LAT is oriented at rocking angles exceeding 52°. We then compare each individual 7-year simulation with the remaining 999 simulations. A fluctuations map in Galactic coordinates with $N_{side} = 64$ is created for each realization, comparing its counts map with the average of the other 999 simulations (i.e., reference map).

Figure 1 shows the APS for the 6 ideal instruments considered with different FoVs. In each plot the 3 colored bands show the regions corresponding to the quantiles at $\pm 1\sigma$, $\pm 2\sigma$ and $\pm 3\sigma$ respectively, calculated from the distribution of the above-mentioned 999 independent APSs at fixed multipole $l$. In the same plot we show the expected values corresponding to the same quantiles calculated from the expectation based on the white noise (average and variance) as discussed in the main text of the paper. The expected white noise and its variance are slightly underestimated at low multipoles ($l \lesssim 5$), in particular for the smaller FoVs considered.

We have repeated the APS calculation with a different number of pixels in the map, and we still observe deviations of the white noise level and its fluctuation with coarse (i.e., $N_{side} = 32$) and fine ($N_{side} = 128$) pixelization. Despite that, we decided to keep the prescription for $C_N$ and its variance as discussed in the main text, but it would be interesting to understand if those deviations can be recovered with a modified analysis (see, e.g., [2]).

We use the same 1000 simulations to check the four analysis methods adopted in the current work. For each simulation we apply the four methods 25 times, and the reference map for each method is calculated averaging these 25 maps. We then calculate the fluctuation map comparing each simulated sky map with its reference map calculated with the four methods, and finally for each method we calculate the APS from the fluctuation map.

Figure 2 (3) shows the APS for the 6 ideal instruments with different FoVs using Method 1 (Method 2) to create

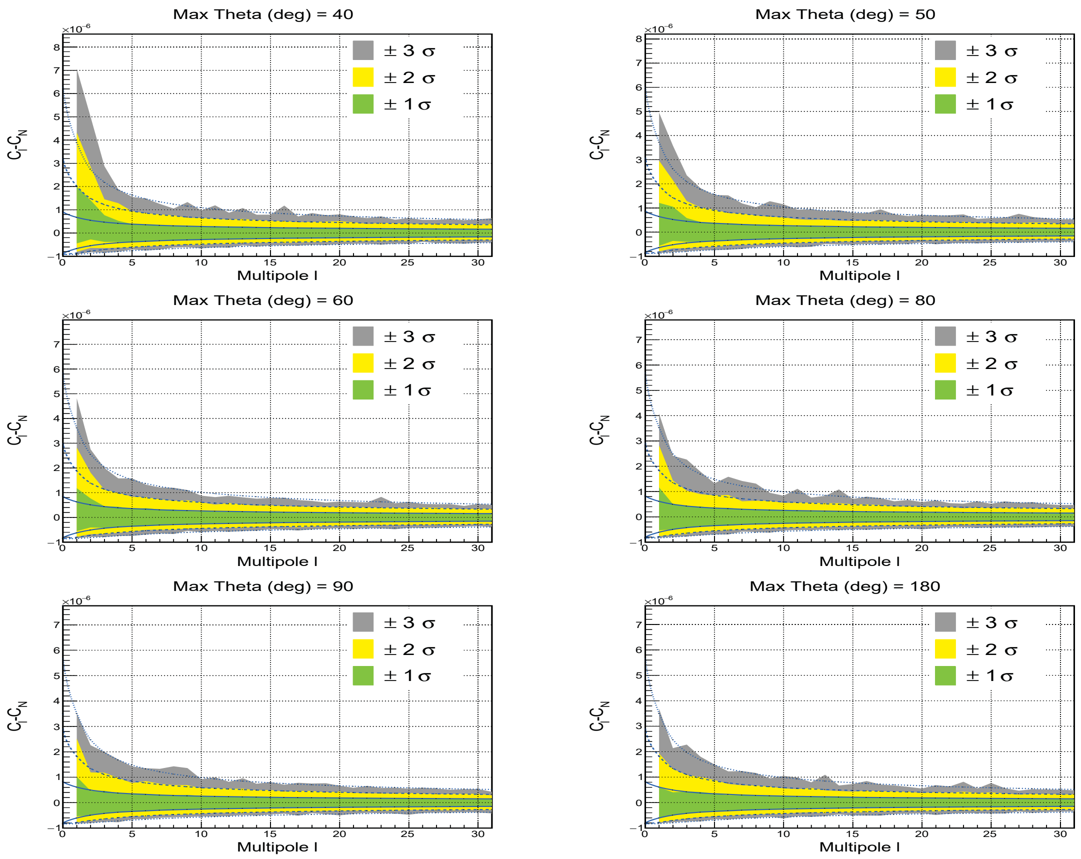


FIG. 1. APS as a function of the multipole $l$ for the six different ideal detectors with different FoVs, using the 1000 independent simulations. The three colored bands show the regions corresponding to different quantiles at $\pm1\sigma$ (green), $\pm2\sigma$ (yellow) and $\pm3\sigma$ (gray) respectively. The blue lines show the expectation based on the knowledge of the white noise distribution at the same quantile values. Note that the fluctuations at around the 3 $\sigma$ level are due to the limited number of simulations.

the reference average map, respectively (Method 3 and 4 are not shown since they give similar results as Method 2 and 1, respectively). In each plot the three colored bands indicate the regions corresponding to different quantiles at $\pm1$, $\pm2$ and $\pm3$ sigma respectively, calculated from the distribution of the above 1000 independent APSs at given multipole $l$.

We note that in these plots the APSs from the fluctuation maps using the reference average map created with Method 1 show some significant bias w.r.t. the white noise level at low multipoles (corresponding to angular scale larger than the FoV). Possibly, the bias could be due to the way in which the time event time sequence is set, which could break the Poisson random process between events on an angular scale larger than the FoV. On the other hand, the reference average map created with Method 2 shows better behaviour w.r.t. the white noise level even with small FoV detectors. The event time sequence in this case is not fixed and it can follow a proper Poisson distribution.

It is worth mentioning that a possible problem with the methods based on the event rate concerns the duration of the time interval used to calculate the all-sky rate in order to have adequate all-sky exposure coverage, particularly in the case of data a sample with limited statistics. In fact, the presence of any small/medium angular scale anisotropies in the data would create transient fluctuations in the instantaneous values of $P(\theta,\phi)$ as these anisotropies pass through the instrument field of view. However, these anisotropies would have no effect on the longer-term average values, since any transient fluctuations would be averaged out [1, 3].

After this simulation campaign with ideal detectors with different FoVs, we decided to apply all four methods to the LAT data for consistency checks of the results.

### Validation of the capabilities of the method to detect a dipole anisotropy

A dedicated validation to test the capabilities of Method 1 and Method 2 to detect a dipole anisotropy was performed. A dipole anisotropy from the direction $(l = 230^{\circ}, b = -3^{\circ})$ with amplitudes 10%, 1%, and 0.1%

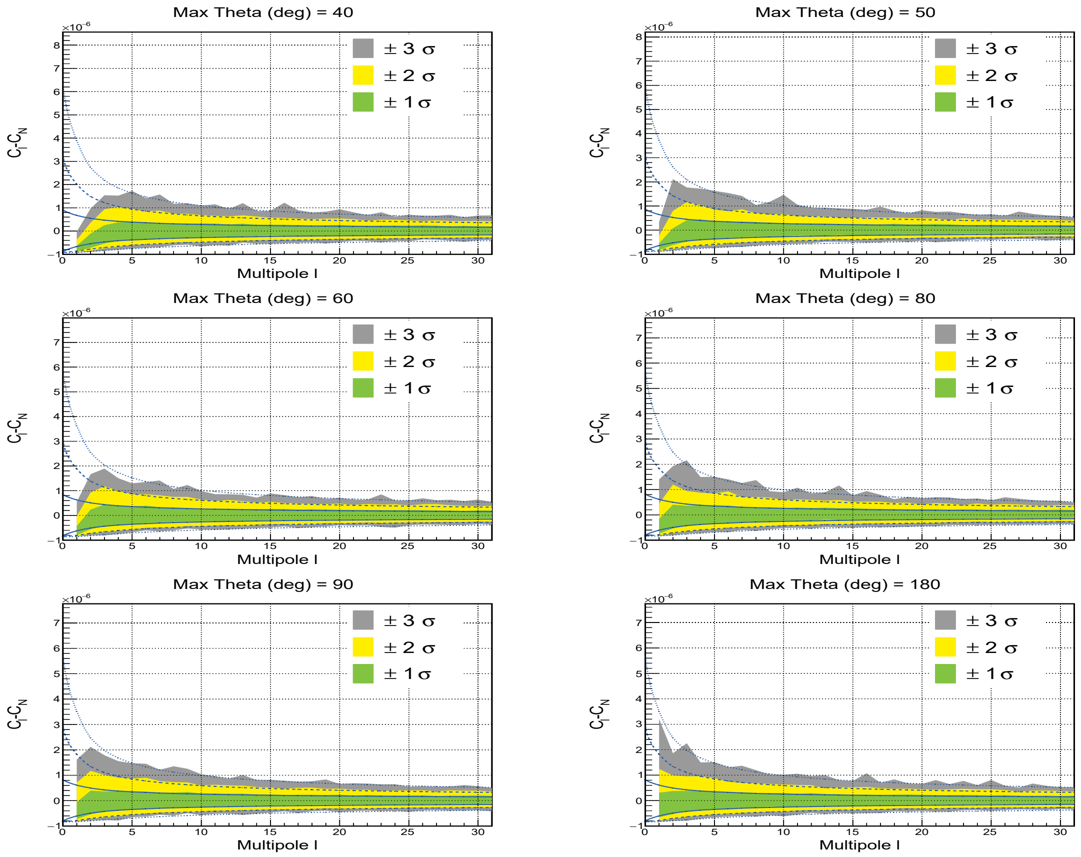


FIG. 2. APS as a function of the multipole $l$ for the six different ideal detectors with different FoVs, using the 1000-independent simulations and Method 1 to create the reference map. The three colored bands show the regions corresponding to different quantiles at $\pm1\sigma$ (green), $\pm2\sigma$ (yellow) and $\pm3\sigma$ (gray) respectively. The blue lines show the expectation based on the knowledge of the white noise and its variance at the same quantile values. Note that the fluctuations at around the 3 $\sigma$ level are due to the limited number of simulations.

was injected in three different simulation sets with an ideal instrument with FoV radius of 60°, each set made of 1000 repetitions. The CRE rate was chosen to simulate $\approx$ 10M events close to the total number of observed events.

Both Method 1 and Method 2 were applied 25 times to each simulation to construct a reference sky map and the dipole strength was calculated from the APS of the fluctuation map as $\delta = 3\sqrt{(C_1 - C_N)/4\pi}$ when $C_1 > C_N$. The measured dipole strength distributions for the two methods and three different levels of dipole anisotropies are shown in Figure 4.

Both methods are able to detect a 10% and 1% dipole anisotropy. Method 2 shows some sensitivity as well to 0.1% dipole anisotropies. Furthermore, Method 1 is significantly biased, detecting a dipole anisotropy that is one third of the value used for simulation, whereas Method 2 shows a better behavior, with a bias of less than 20%.

## OPTIMIZATION OF EVENT SELECTION

Assuming an isotropic distribution of charged particles at very large distances from the Earth, not all of these particles are able to reach the LAT due to the action of the geomagnetic field and Earth's shadow. Any particle reaching the detector must come from an allowed direction, with the set of allowed directions depending on the location of Fermi spacecraft in orbit point and on the particle energy and charge.

In the case of CREs there are pure-positron and pure-electron regions in the West and in the East, respectively, where only positrons or electrons are allowed. The sizes of these regions depend on the particle energy and on the instrument position. As the energy increases, the sizes of both regions decrease. Since the CRE sample is mainly composed of electrons with a small fraction of positrons and a small possible proton contamination, the presence of particles with different charge signs could introduce additional features because the allowed regions are different. To study the geomagnetic effect on the

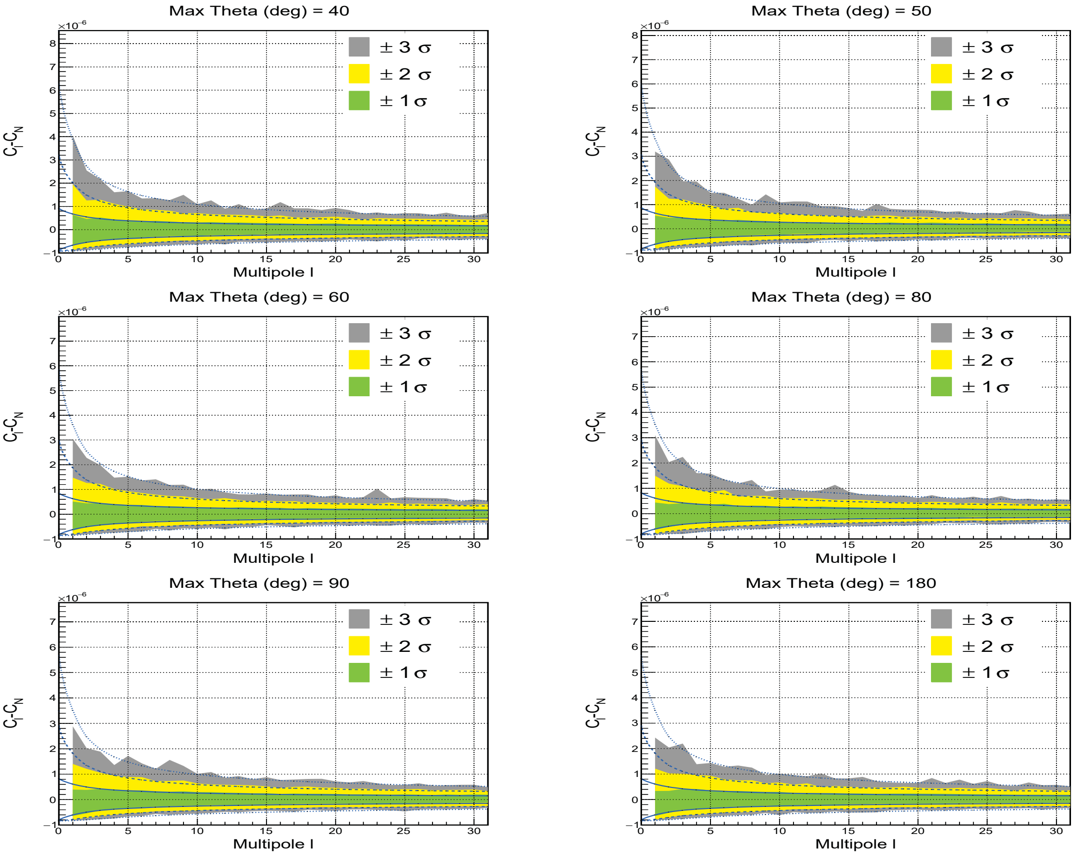


FIG. 3. Same as Fig. 2, but using Method 2 to create the reference map.

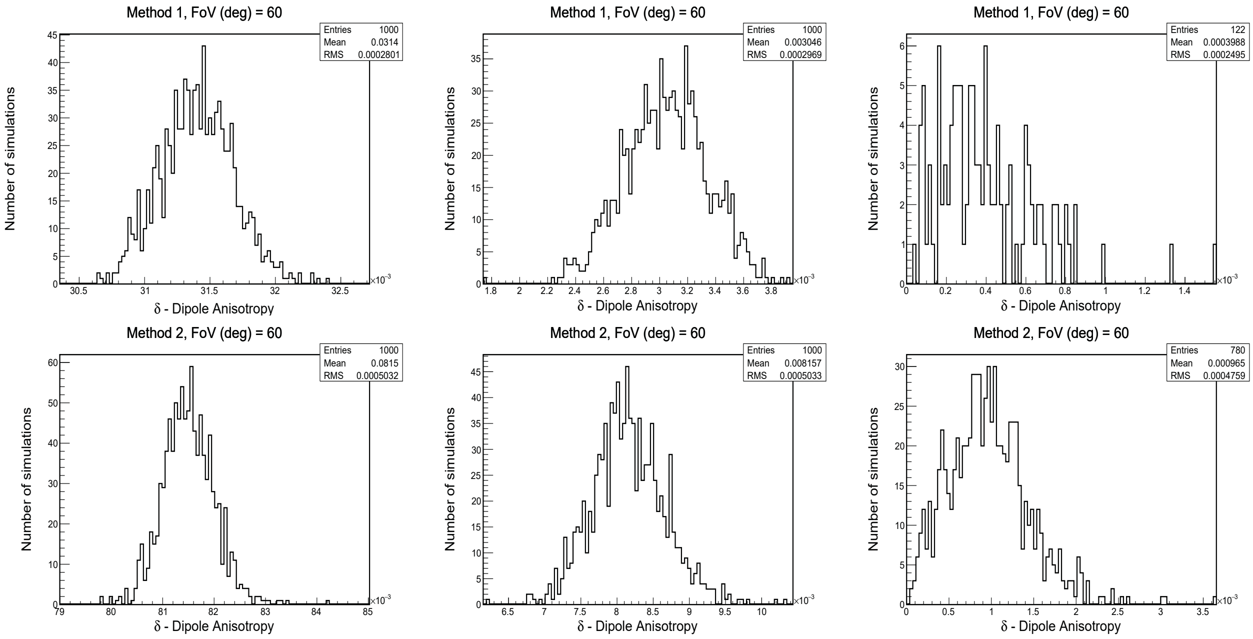


FIG. 4. Dipole anisoptropy distributions as measured in the simulations with 10%, 1%, and 0.1% dipole anisotropy are shown in columns from left to right. Method 1 (Method 2) was used for the generation of the reference sky map used in the top (bottom) row. The number of entries in each histogram corresponds to those simulation with $C_1 > C_N$.

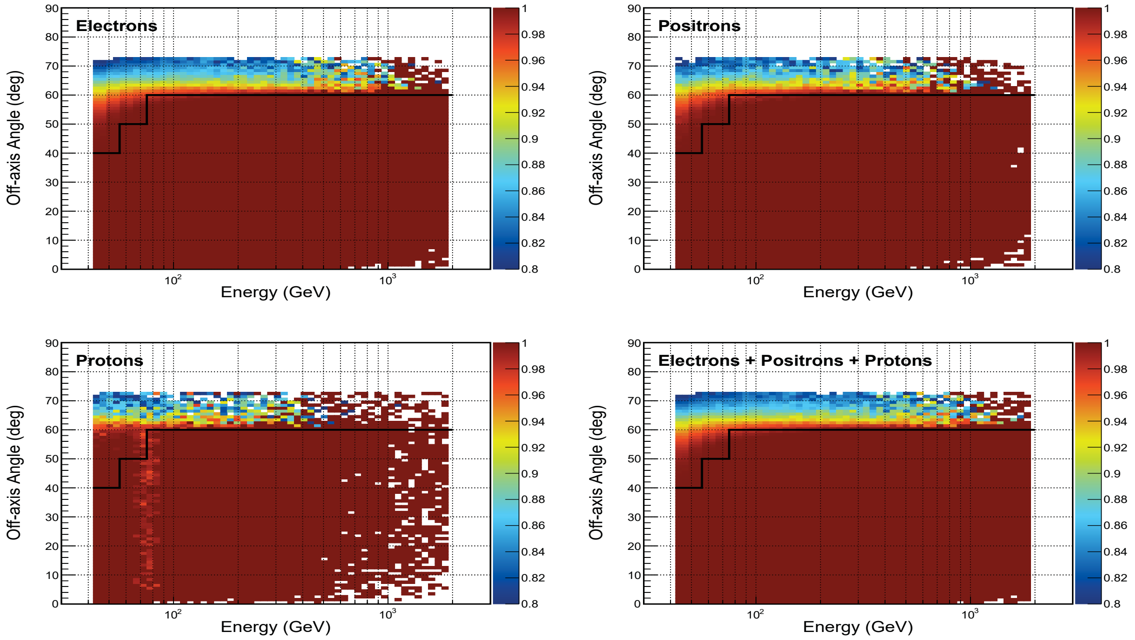


FIG. 5. Ratio of allowed events to total events as a function of the off-axis angle and energy. Top left: Electrons; top right: Positrons; bottom left: Protons; bottom right: Electrons + Positrons + Protons. The black solid line shows the maximum allowed off-axis angle in the event selection.

arrival directions of CREs detected by the LAT we developed a dedicated simulation.

The simulation begins with the IRFs [4] for pure electron, positron, and proton samples in which we apply the set of event selections to identify the electrons [4]. In the simulation we include both energy and angular dispersion effects. We simulate an isotropic distribution in the LAT of electrons, positrons and protons. The the position and orientation of the LAT is taken from real data.

Any detected particle, according to the IRF, is back-tracked in the geomagnetic field (with inverted charge sign) from the LAT to 10 Earth radii to check whether it is trapped in the magnetic field or blocked by the Earth (forbidden direction). The Earth is defined as a sphere with radius given by the average Earth's radius plus 70 km to account for Earth's atmosphere. We used the International Geomagnetic Reference Field (IGRF-12) model [5] to describe the magnetic field in the proximity of the Earth. The CR intensities are taken from the AMS02 data (protons from [6], electrons and positrons from [7]).

We start by selecting GTIs when the LAT is in standard operation outside the SAA region in sky survey mode and removing the times when the LAT is oriented at rocking angles exceeding 52°. This selection helps to remove observation times at high zenith angles (at the Fermi satellite orbit altitude of about 550 km the limb of the Earth is seen at a zenith angle of about 110°), but additional requirements are needed to remove regions affected by the East-West effect.

In fact, charged cosmic rays are deflected by the Earth's magnetic field and, in particular, positive (negative) cosmic rays from the East (West) are suppressed compared to those from the West (East), because the presence of the Earth effectively shadows certain trajectories, which are therefore forbidden. In addition, low-energy cosmic rays can be trapped by the geomagnetic field and so cannot reach the LAT from very large distances from the Earth. These particles may introduce some features in the arrival directions, creating an asymmetry in the (azimuth, zenith) distribution for any given position of the LAT.

Figure 5 shows the ratio between the number of events incident the LAT and the total number of events as a function of the off-axis angle and energy. We show this ratio for the individual particle species (electron, positron and proton contamination) and for their sum. These plots indicate we can see some deficits at large off-axis angle due to particles that are not allowed to reach the LAT. These events come from large zenith angles as shown in Fig. 6, in particular negatively (positively) charged particles are suppressed from East (West) as expected. We calculate the fractions of total events in the allowed/forbidden regions and we set the maximum off-axis angle to reduce any features that could mimic true anisotropies below the actual sensitivity. The maximum off-axis angle as a function of the energy is shown with a

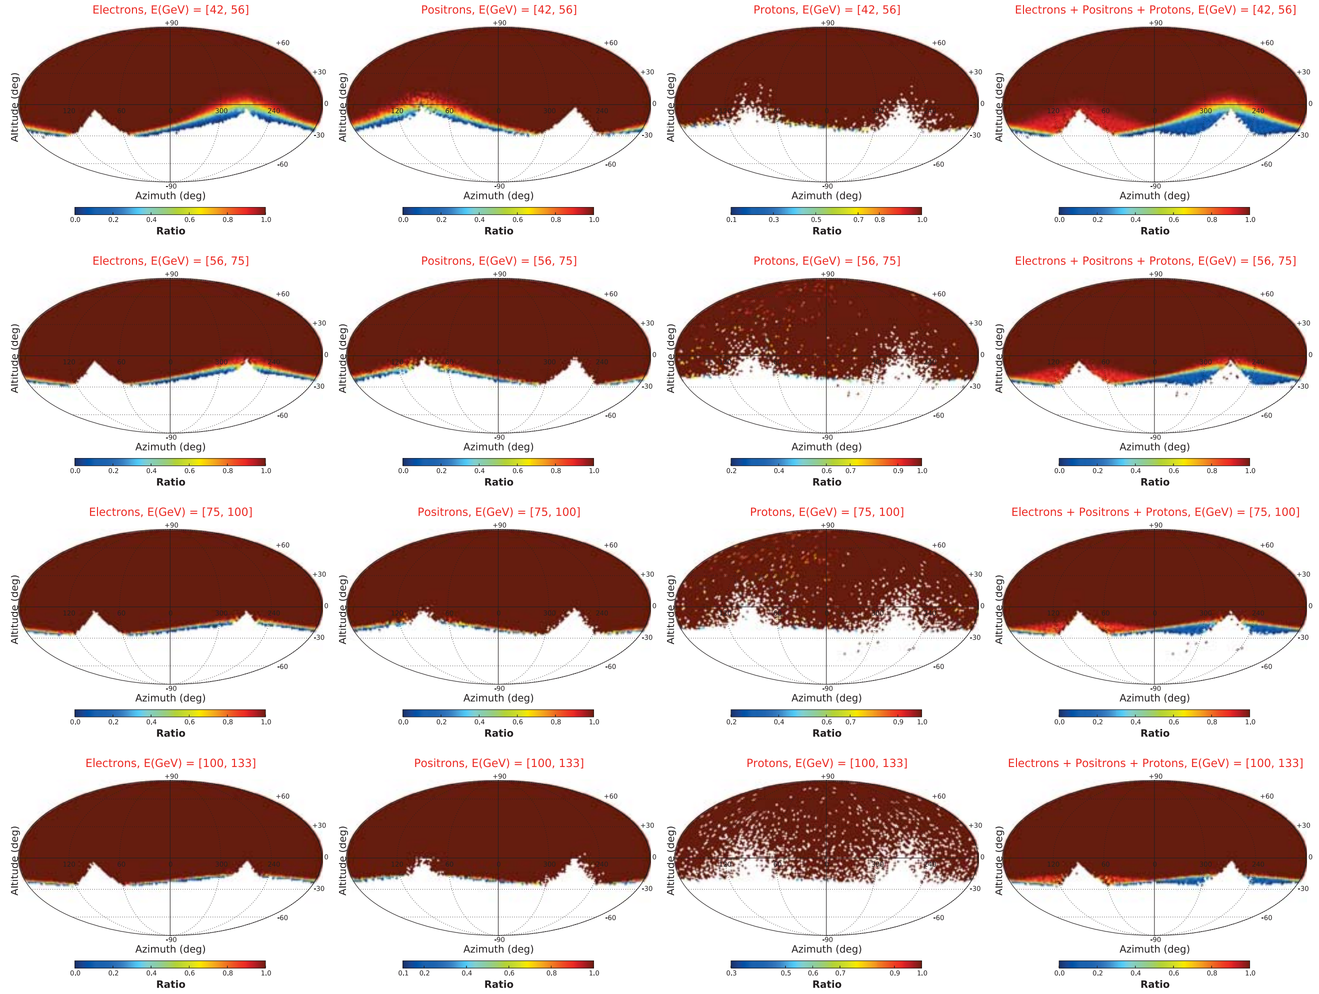


FIG. 6. Allowed events to the total event ratio map in zenith-centered coordinates (Mollweide projection), for different energy bins, from 42 GeV (top) to 133 GeV (bottom). Left: Electrons; middle left: Positrons; middle right: Protons; right: Electrons + Positrons + Protons.

black line in Fig. 5.

The effect of the cut on the off-axis angle is to reduce the zenith angle interval observed by the LAT (see Fig. 7). In this way, the forbidden regions have been removed without introducing any asymmetry in the instrument coordinate system. In Fig. 7 we also show for the nine energy bins the reference maps created with Method 2 and the significance. We evaluate the significance by comparing the counts for each pixel between the simulated maps and the reference maps following the prescriptions of Ref. [8]. We use the likelihood ratio method of Ref. [8] to evaluate the significance, and a positive (negative) sign of the significance is chosen in the case of excess (deficit) of the actual counts w.r.t. the reference map.

## VALIDATION WITH A MORE REALISTIC SIMULATION

The simulation described in the previous section is used to check Method 1-4 to create the reference sky maps. We calculated the APS of the fluctuation maps created with the four methods discussed above. For Method 2 and Method 3 we calculate the rate using a time interval of about two months. For each method we average 10000 realizations to create the average reference map to be used to extract the APS. Figs. 8 and 9 show the counts and the average reference sky maps of simulated data, respectively.

The APS is shown in Fig. 10 for each of the nine energy bins in the range of multipoles of interest of this analysis, i.e., up to $l = 30$. The APS has been calculated on the fluctuation maps with $N_{side} = 64$. We also show the APS for each energy bin over a broader multipole range up to

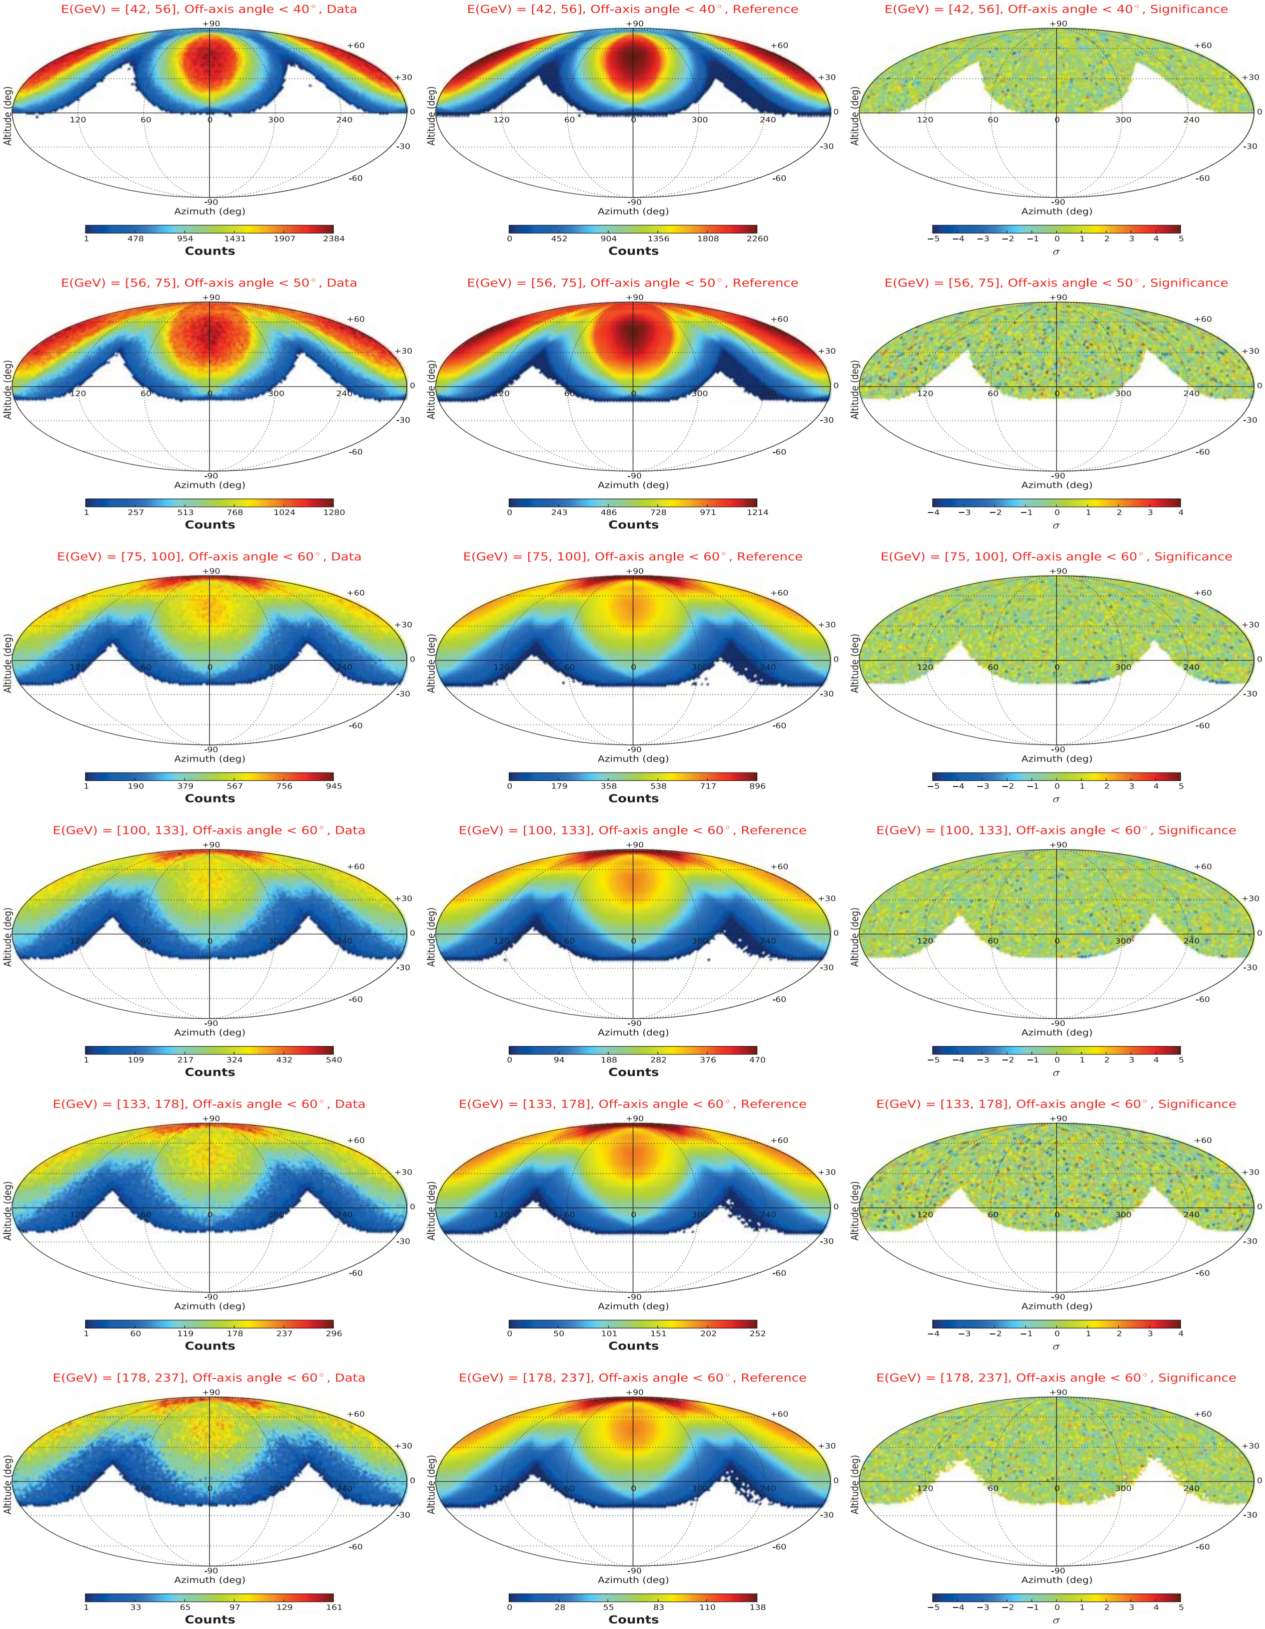


FIG. 7. Simulated CRE data map (left column), reference map (middle column) and significance map (right column) for the nine energy bins in zenith-centered coordinates (Mollweide projection).

$l = 191$, i.e., $l = 3 \times N_{side} - 1$, in Fig. 11. The markers in Figs. 10 and 11 show the evaluated APS with the white

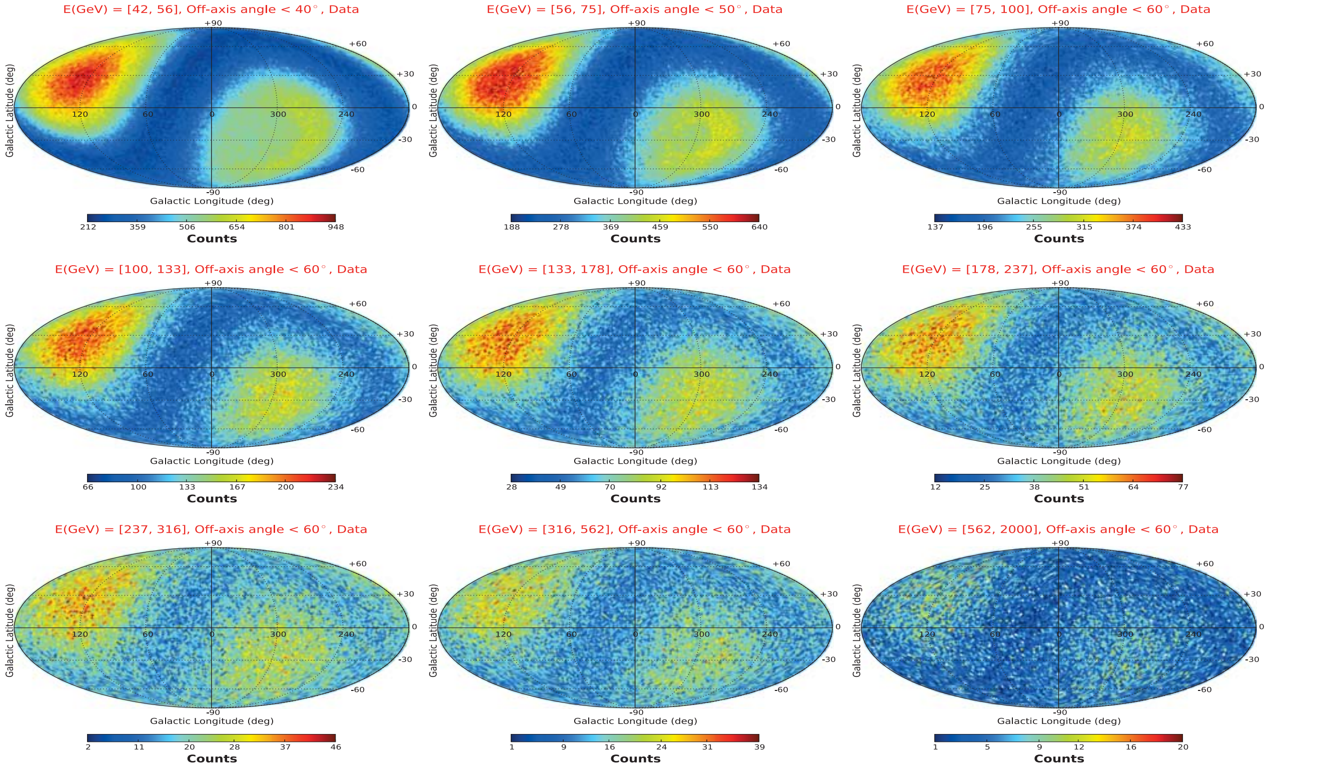


FIG. 8. Simulated data sky maps for the nine energy bins in Galactic coordinates (Mollweide projection).

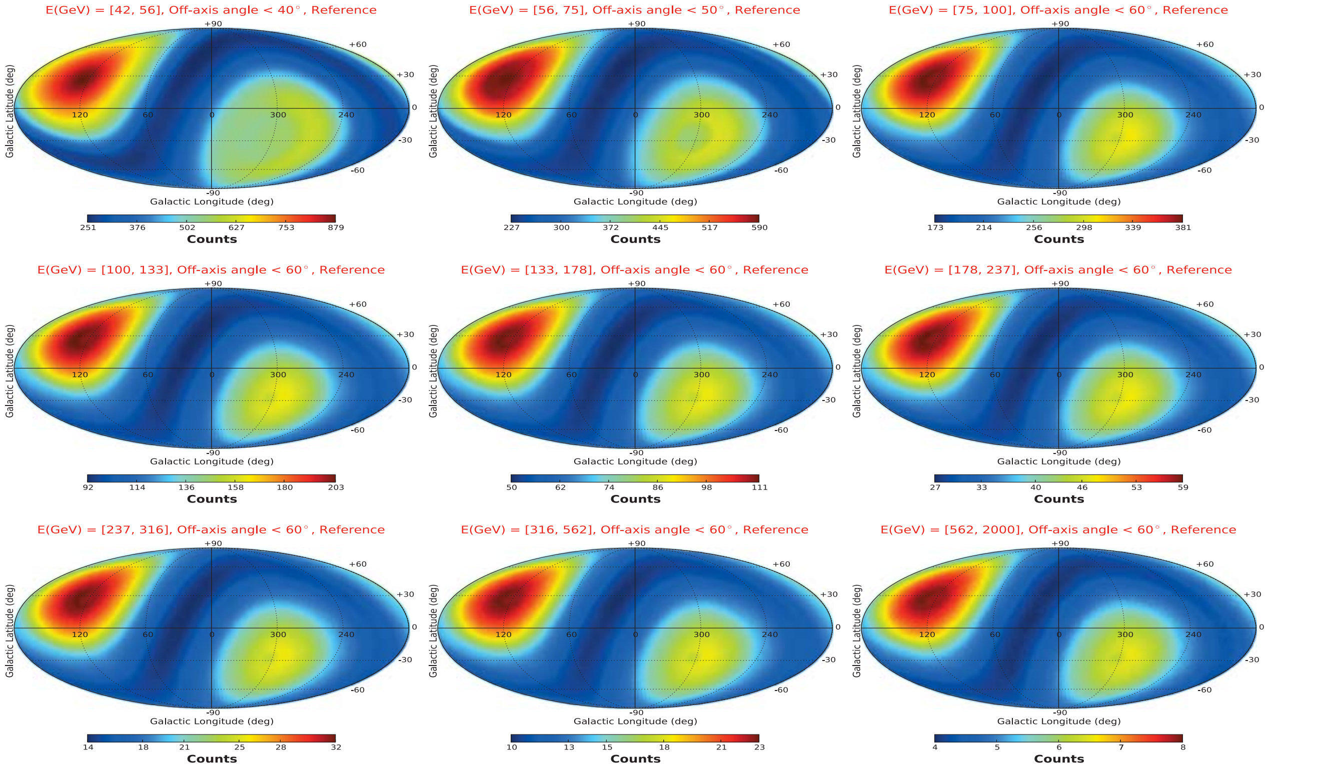


FIG. 9. Reference sky maps for the simulated data for the nine energy bins in Galactic coordinates (Mollweide projection).

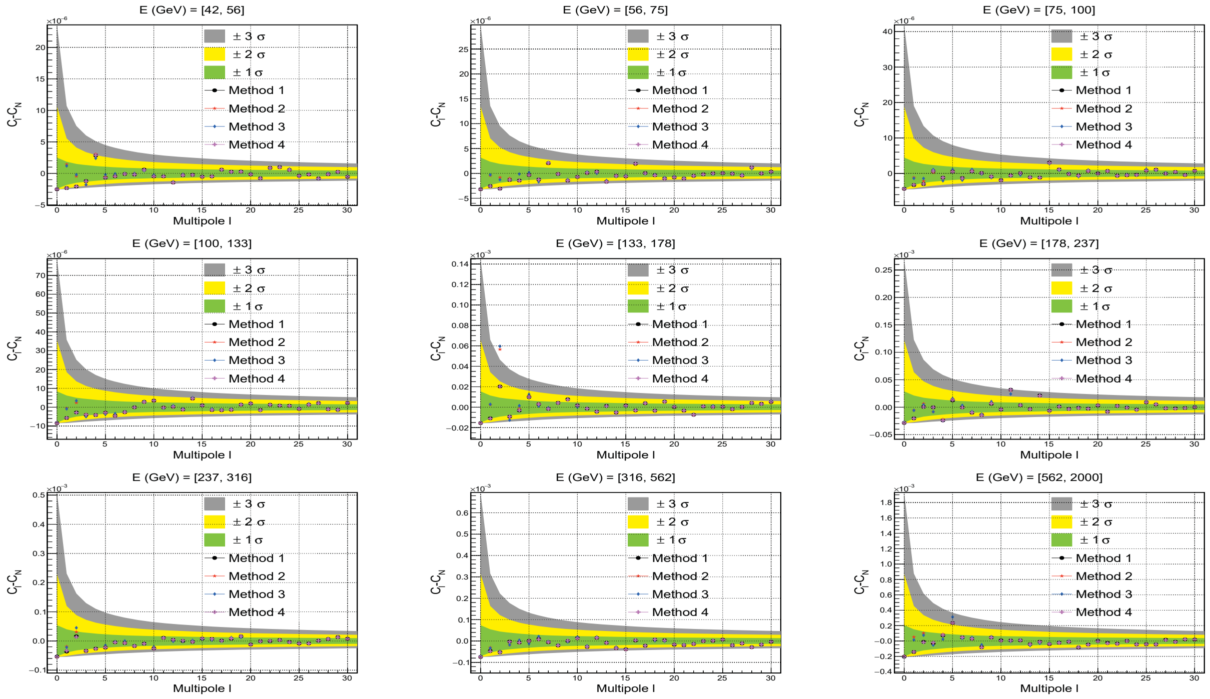


FIG. 10. APS for the CRE simulated data in the nine energy bins using Methods 1-4 to create the reference maps. The markers in the figures show the produced APS with the white noise spectrum subtracted. The colored bands in the same figure show the range of the statistical fluctuations of the white-noise power spectrum ($C_N$) for different confidence intervals, i.e., $\pm 1\sigma$ (green), $\pm 2\sigma$ (yellow) and $\pm 3\sigma$ (gray) level respectively.

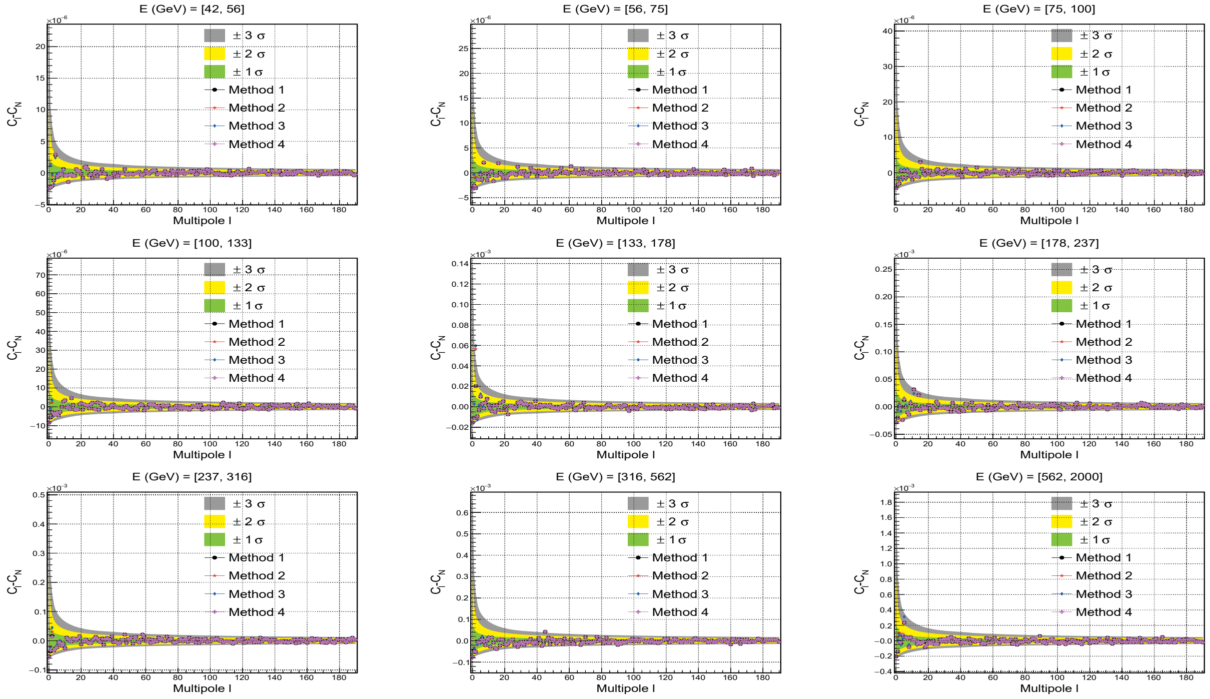


FIG. 11. Same as Fig. 10, but showing a wider range in multipole.

noise spectrum subtracted, i.e., they show $C_l - C_N$. The colored bands in the same figure show the range of the statistical fluctuations of the white noise power spectrum for different confidence intervals. i.e., $\pm 1$, $\pm 2$ and $\pm 3$ $\sigma$

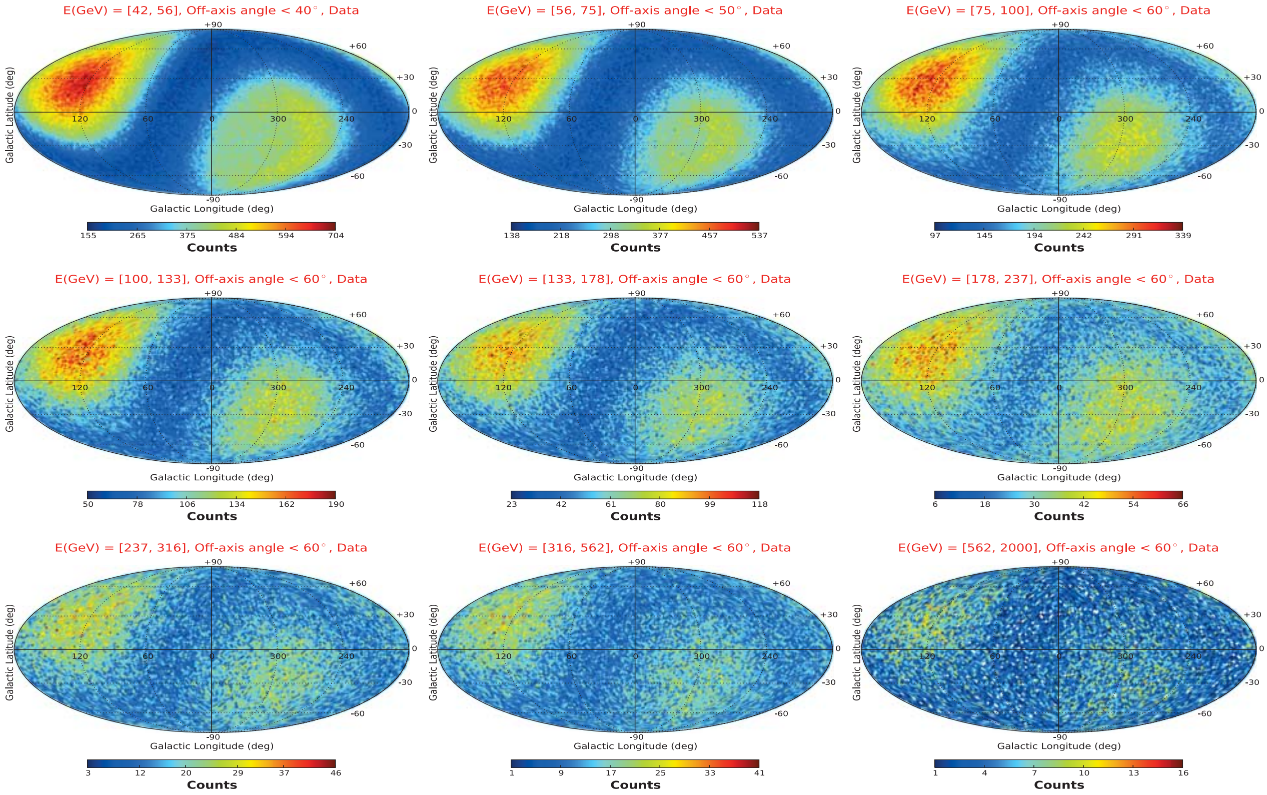


FIG. 12. Real data sky maps of CREs for the nine energy bins in Galactic coordinates (Mollweide projection).

level. All data points (markers) for both methods lie within the $3\sigma$ range, demostranting that both methods do not introduce features when reconstructing the no-isotropic sky map.

As already shown in the main text (see Fig. [2]), Methods 1 and 4 show some bias w.r.t. the white noise level at dipole angular scale for the low energy bins (i.e., the ones with smaller FoVs), while Methods 2 and 3 show a better behavior w.r.t. the white noise level expectation. These results are similar to the one discussed above with ideal detector with different FoVs. However, the dipole anisotropies for Methods 1-4 are within the confidence belt set by the white noise.

## SKY MAPS AND APS FOR LAT DATA

Here we present the results with real data. As discussed above, we perform the analysis in nine independent energy bins with an energy-dependent FoV as described before. We show the sky maps of the events selected for the current analysis in Galactic coordinates in Fig. 12. Figure 13 shows the maps in Horizontal coordinates. In this figure we show the real counts maps, the reference maps created with Method 2 and the significance maps obtained comparing pixel-by-pixel the real and the refereence map counts.

Figure 14 shows the significance sky maps in Galactic coordinates obtained by comparing the integrated reference sky maps produced with Method 2 to the actual integrated sky maps (10, 30, 45, 60 and 90 degrees circular region size). The significances shown in these maps are pre-trials, i.e., they do not take into account the correlations between adjacent pixels (see [1] for a full discussion). None of these maps indicates significant excesses or deficits at any angular scale, showing that our measurements are consistent with an isotropic sky.

We then calculate the APS with the shuffling (Method 1) and the event rate (Method 2) methods. The APS is shown in Fig. 15 for each of the nine energy bins as a function of multipole $l$ up to 30. The APS has been calculated on the fluctuation maps with $N_{side} = 64$. We also show the APS in Fig. 16 for each energy bin over a broader multipole range up to $l = 191$, i.e., $3 \times N_{side} - 1$. The markers in those figures show the calculated APS with the white noise spectrum subtracted, i.e., they show $C_l - C_N$. The colored bands in the same figure show the range of the statistical fluctuations of the white-noise power spectrum ($C_N$) for different confidence intervals, i.e., $\pm 1$, $\pm 2$ and $\pm 3$ $\sigma$ level. All the data points (markers) for both methods lie within the $3\sigma$ range, showing the consistency with an isotropic sky.

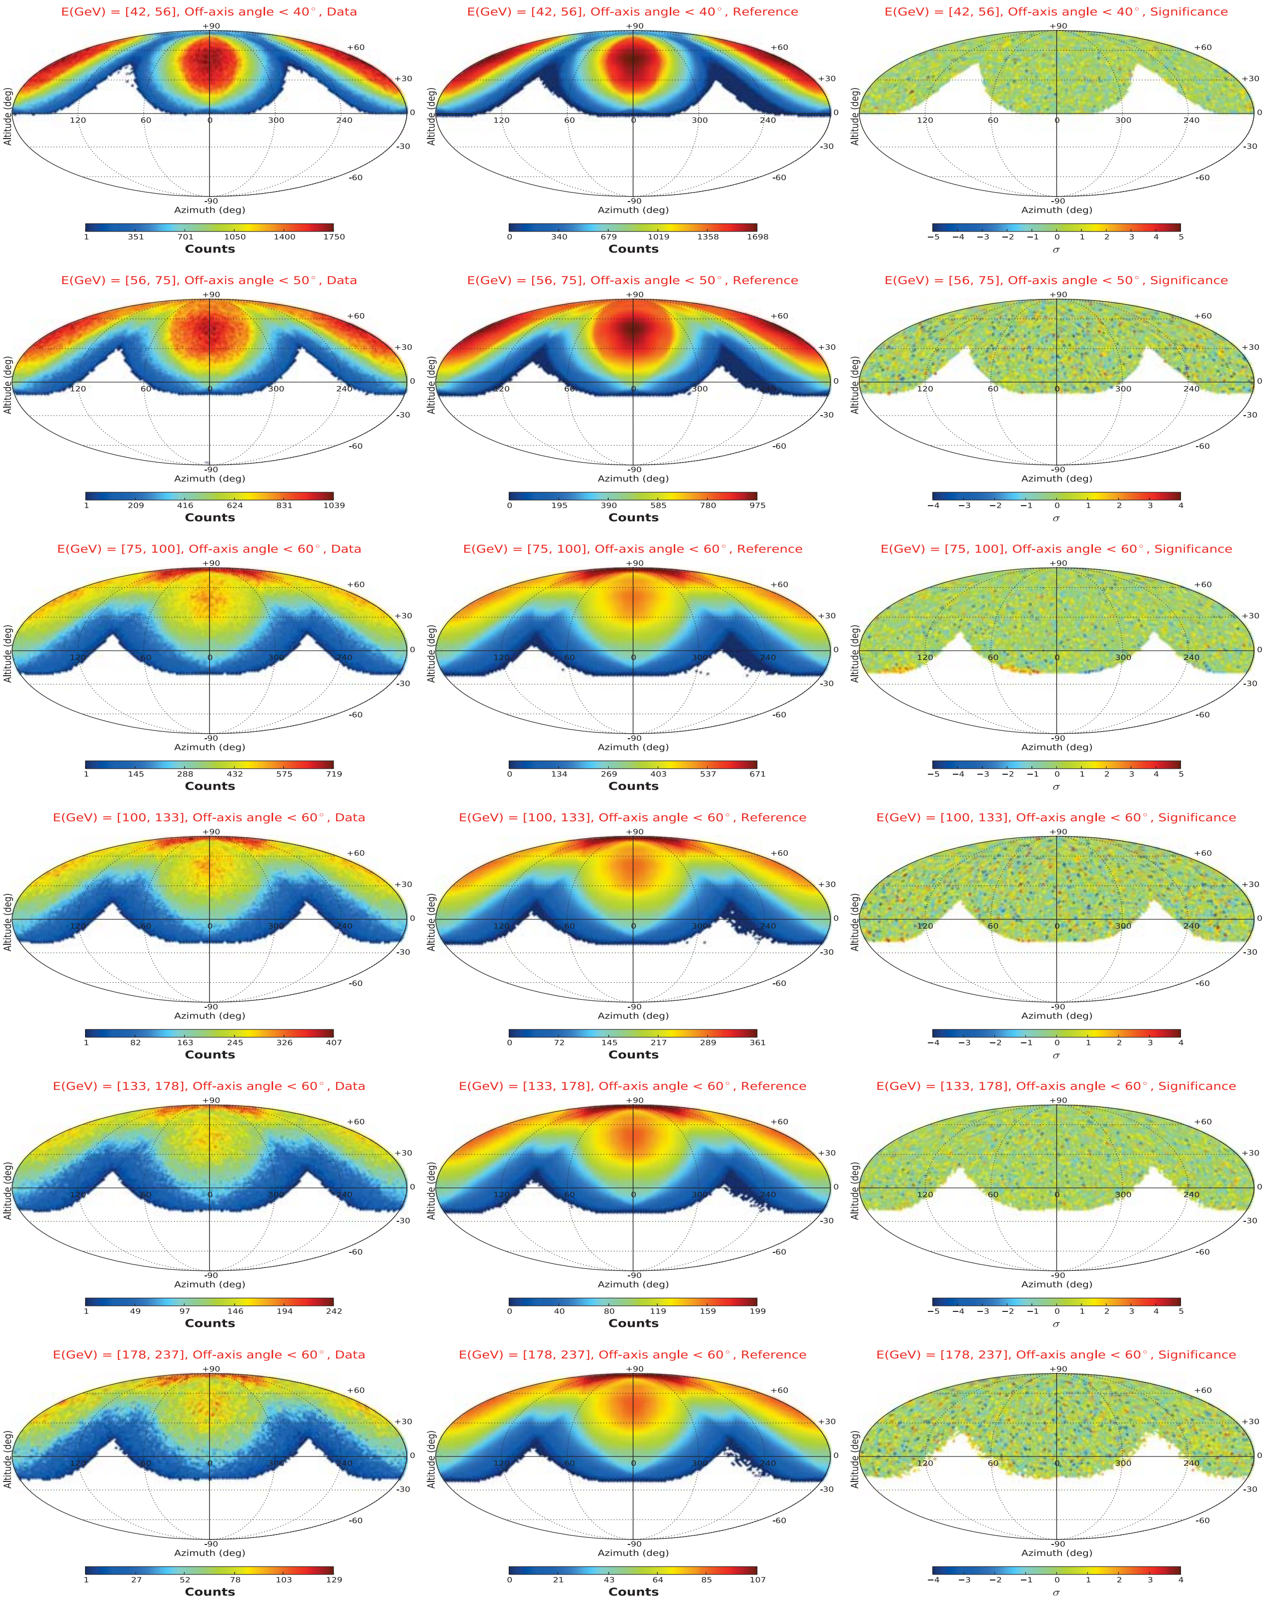


FIG. 13. Real data map (left column), reference map (middle column) and significance map (right column) of CREs for the nine energy bins in Horizontal coordinates (Mollweide projection).

### UPPER LIMIT ON THE DIPOLE ANISOTROPY

The power spectrum characterizes the intensity fluctuations as a function of the angular scale. The data (raw $C_l$ calculated with `anafast`) can be regarded as the sum of two independent components; an anisotropic one, which we aim to detect, and an isotropic one, which is known and equivalent to the white noise. Since the two components are not correlated, the APS can be similarly split into two components, i.e.: $\hat{C}_l = \hat{C}_l^{ani} + \hat{C}_l^N$. The quantities $C_l$, $C_l^{ani}$, and $C_l^N$ are random variables (i.e., outcomes), in general different from their true underlying quantities $\hat{C}_l$, $\hat{C}_l^{ani}$ and $\hat{C}_l^N$ respectively.

The expected white noise (maximum likelihood estimator) $C_N$ of $\hat{C}_l^N$ is:

$$< \hat{C}_l^N >= C_N = \frac{4\pi}{N_{pixels}^2} \sum_{i=1}^{N_{pixels}} \frac{n_i}{\mu_i^2} \quad (1)$$

where $n_i$ is the number of events in the $i-th$ pixel and $\mu_i$ is the expected number of events in that pixel, taking into account the instrument exposure (from the reference map) [9].

The quantity $\hat{C}_l$ follows a $\chi^2_{2l+1}$ distribution with variance $var(\hat{C}_l) = \frac{2}{2l+1}(C_N + \hat{C}_l^{ani})^2$. To search for anisotropies in the data, we tested the null hypothesis, i.e., $\hat{C}_l^{ani} = 0$ or equivalently $\hat{C}_l = C_N$. This was accomplished by checking whether the observed power spectrum $\hat{C}_l$ was statistically compatible with the known true value of the isotropic power spectrum $C_N$.

The resulting power spectra can be used for setting upper limits on the degree of anisotropy:

$$\delta \equiv \frac{I_{max} - I_{min}}{I_{max} + I_{min}}, \quad (2)$$

where $I_{max}$ and $I_{min}$ are the maximum and minimum values of the CRE intensity. Consider a dataset consisting of the sum of a perfectly isotropic signal of constant intensity $I_0$ and of a dipole anisotropy of maximum intensity $I_1$. The overall intensity at an angular distance $\theta$ from the maximum of the dipole anisotropy will be $I(\theta) = I_0 + I_1 \cos\theta$. For this dataset, the degree of its dipole anisotropy is

$$\delta = \frac{I_1}{I_0}. \quad (3)$$

The fluctuation map describing this dataset is:

$$f(\theta) = \frac{I(\theta) - < I(\theta) >}{< I(\theta) >} = \frac{I(\theta) - I_0}{I_0} = \frac{I_1}{I_0} \cos\theta. \quad (4)$$

Since $Y_1^0(\theta, \phi) = \sqrt{\frac{3}{4\pi}} \cos\theta$, it follows from Eq. 4 that $f(\theta) = \left( \frac{I_1}{I_0} \sqrt{\frac{4\pi}{3}} \right) \times Y_1^0$ or equivalently

$$a_{10} = \frac{I_1}{I_0} \sqrt{\frac{4\pi}{3}}. \quad (5)$$

All but the $l = 1$ term of the power spectrum will vanish. The only non-zero term is:

$$C_1 \equiv \frac{1}{3} \sum_{m=-1}^{1} |a_{1m}|^2 = \frac{a_{10}^2}{3} = \left( \frac{I_1}{I_0} \right)^2 \frac{4\pi}{9}. \quad (6)$$

It should be noted that since $C_1$ is a rotationally invariant quantity, the above expression for $C_1$, derived in the reference frame where $a_{11} = 0$ and $a_{1-1} = 0$, has general validity. From Eqs. 3 and 6 a relation between the degree of dipole anisotropy and the value of the dipole power can be derived:

$$\hat{\delta} = 3 \sqrt{\frac{\hat{C}_1^{ani}}{4\pi}}. \quad (7)$$

To set an upper limit (UL) on $\hat{\delta}$ we start by calculating the UL on $\hat{C}_1^{ani}$ from the probability distribution function (pdf) of $C_1$; then the corresponding limit for $\hat{\delta}$ can be calculated from Eq. 7.

The probability of observing a value of $C_1$ (raw value calculated with `anafast`) given the true dipole power $\hat{C}_1$ is:

$$P(C_1 | \hat{C}_1^{ani}, C_N) = \frac{3\sqrt{3}}{\sqrt{2\pi} \hat{C}_1} \sqrt{\frac{C_1}{\hat{C}_1}} \exp\left( -\frac{3C_1}{2\hat{C}_1} \right) \quad (8)$$

where $\hat{C}_1 = \hat{C}_1^{ani} + C_N$.

The limit for $\hat{C}_1^{ani}$ at a given confidence level (for the frequentist approach) or credibility interval (for the Bayesian approach) can be calculated using the likelihood ratio method or the posterior probability method respectively. The methods described below have been subjected to a coverage study to check the exepcted confidence levels.

#### Frequentist confidence intervals

The expected value (maximum likelihood estimator) of $\hat{C}_1^{ani}$ ($\hat{\hat{C}}_1^{ani}$) can be calculated from Eq. 8 by solving the equation

$$\frac{\partial \ln P(C_1 | \hat{C}_1^{ani}, C_N)}{\partial \hat{C}_1^{ani}} = 0 \quad (9)$$

where

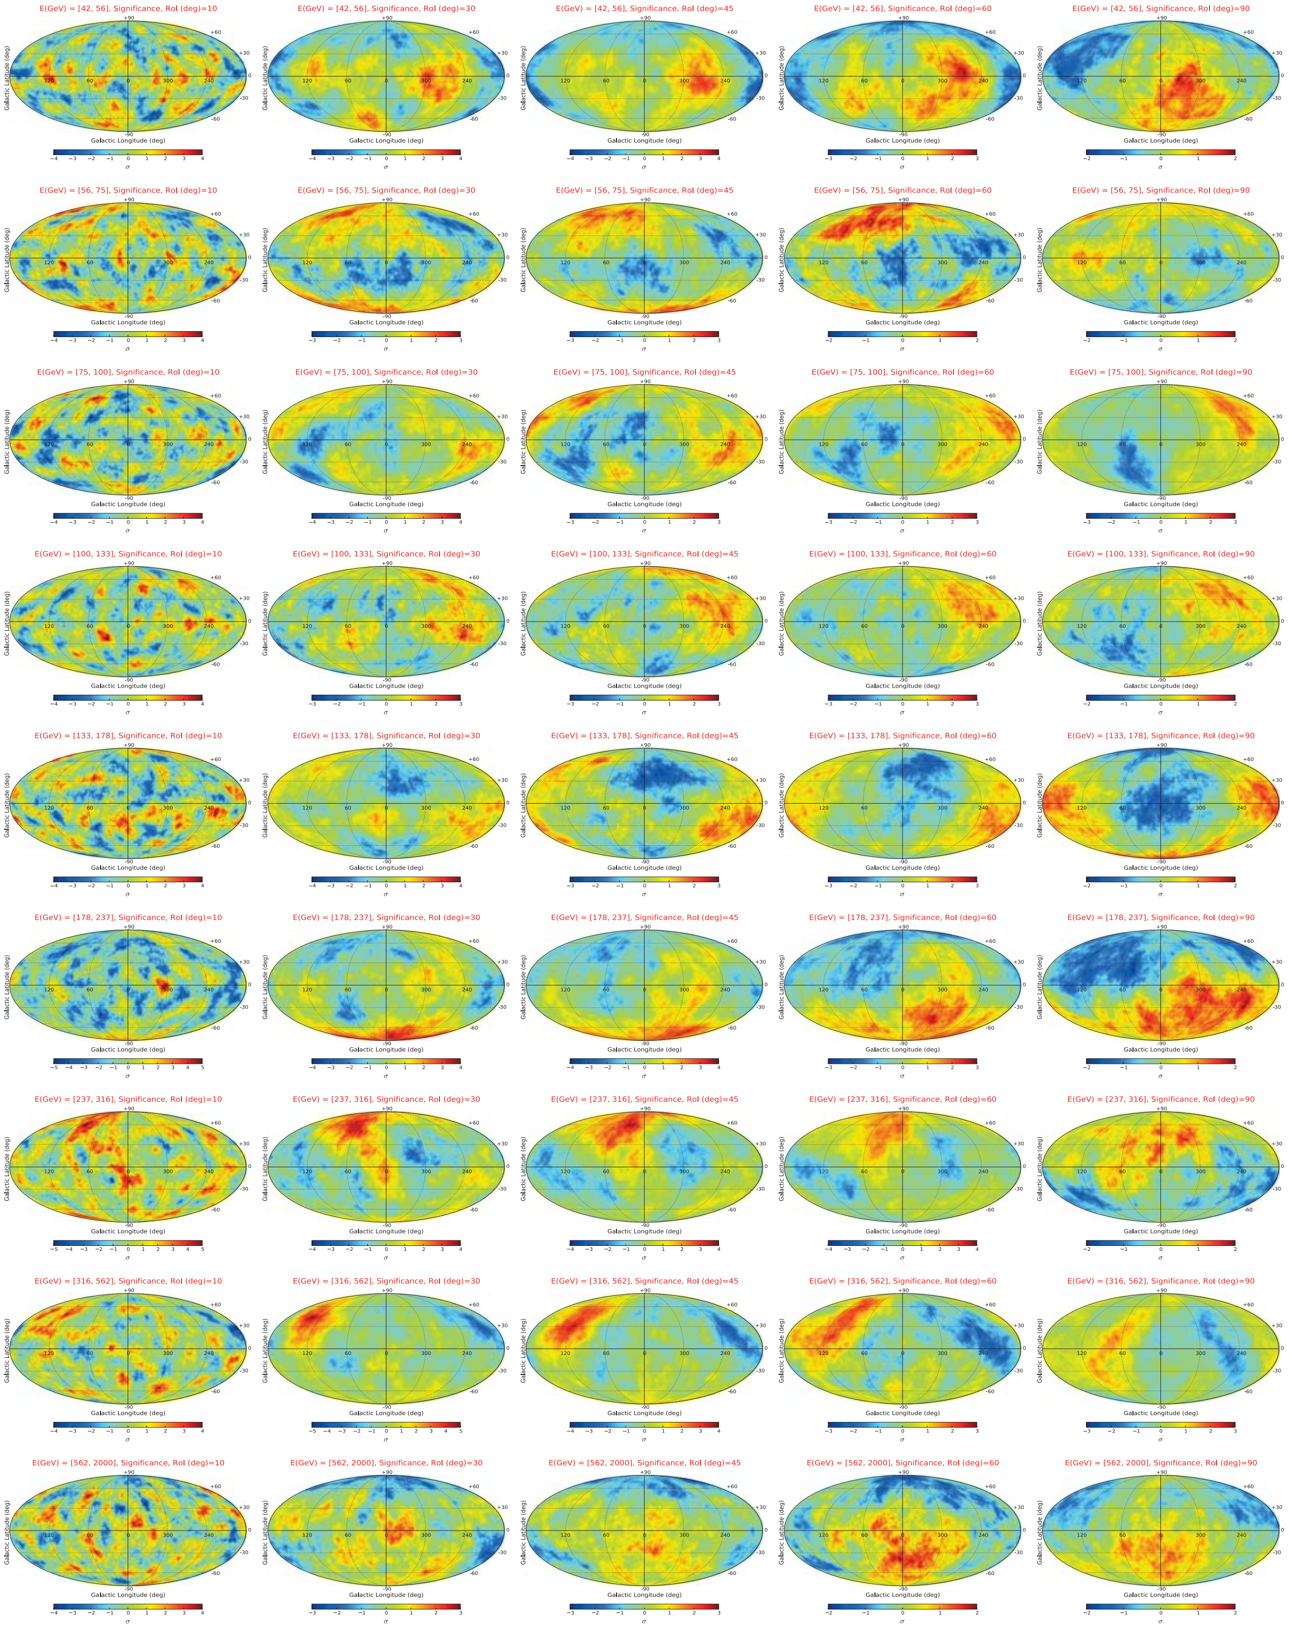


FIG. 14. Significance maps in Galactic coordinates (Mollweide projection) for the nine energy bins and for different integration radii, i.e., 10, 30, 45, 60 and 90 degrees from left to right. The significance has been calculated by comparing the map of real data with the reference map produced by Method 2.

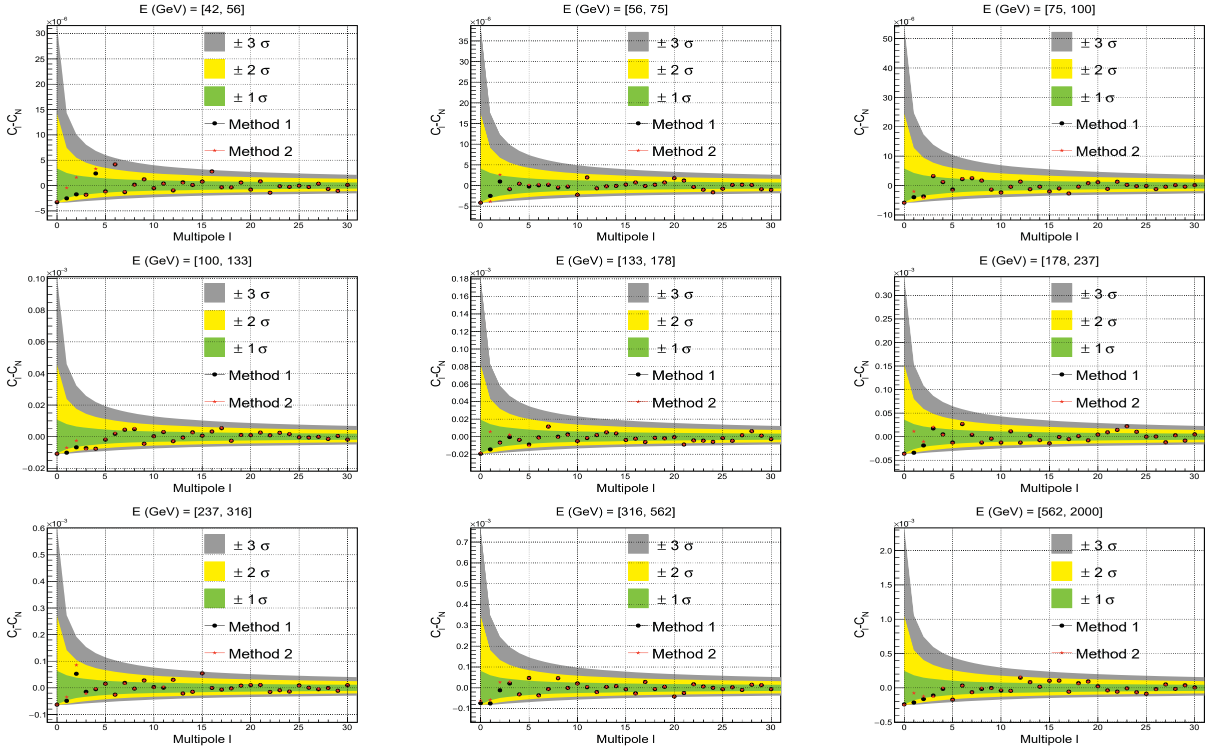


FIG. 15. APS for the real CRE data in the nine energy bins using Methods 1 and 2 to create the reference maps. The markers in the figures show the produced APS with the white noise spectrum subtracted. The colored bands show the range of the statistical fluctuations of the white-noise power spectrum ($\hat{C}_N$) for different confidence intervals, i.e., $\pm 1\sigma$ (green), $\pm 2\sigma$ (yellow) and $\pm 3\sigma$ (gray) level respectively.

$$\ln P = -\frac{3}{2}\left(\ln\left(\hat{C}_1^{ani} + C_N\right) + \frac{C_1}{\hat{C}_1^{ani} + C_N}\right) + c \quad (10)$$

where $c$ is a constant term that does not depend on $\hat{C}_1^{ani}$. By requiring $\hat{C}_1^{ani} \geqq 0$ it follows that:

$$\hat{\hat{C}}_1^{ani} = \begin{cases} C_1 - C_N & \text{if } C_1 - C_N > 0 \\ 0 & \text{otherwise} \end{cases} \quad (11)$$

To calculate the limit for $\hat{C}_1^{ani}$ at a given confidence level (CL), a test statistic based on the likelihood ratio can be used:

$$\lambda = \frac{P(C_1|\hat{C}_1^{ani}, C_N)}{P(C_1|\hat{\hat{C}}_1^{ani}, C_N)} \quad (12)$$

The quantity $-2\ln\lambda(\hat{C}_1^{ani})$ follows a $\chi^2$ distribution with one degree of freedom, i.e., $-2\ln\lambda \sim \chi^2(1)$:

$$-2\ln\lambda(\hat{C}_1^{ani}) = \begin{cases} 3\left(\ln\frac{\hat{C}_1^{ani}+C_N}{C_1} + \frac{C_1}{\hat{C}_1^{ani}+C_N} - 1\right) & \text{if } C_1 - C_N > 0 \\ 3\left(\ln\frac{\hat{C}_1^{ani}+C_N}{C_N} + \frac{C_1}{\hat{C}_1^{ani}+C_N} - \frac{C_1}{C_N}\right) & \text{otherwise} \end{cases} \quad (13)$$

The limit at a given confidence interval of $\hat{C}_1^{ani}$ can be calculated assuming a $\Delta\chi^2$ for that coverage probability; for example, the limit at 95% CL corresponds to a $\Delta\chi^2 = 3.84$. Once the limit on $\hat{C}_1^{ani}$ is known, the

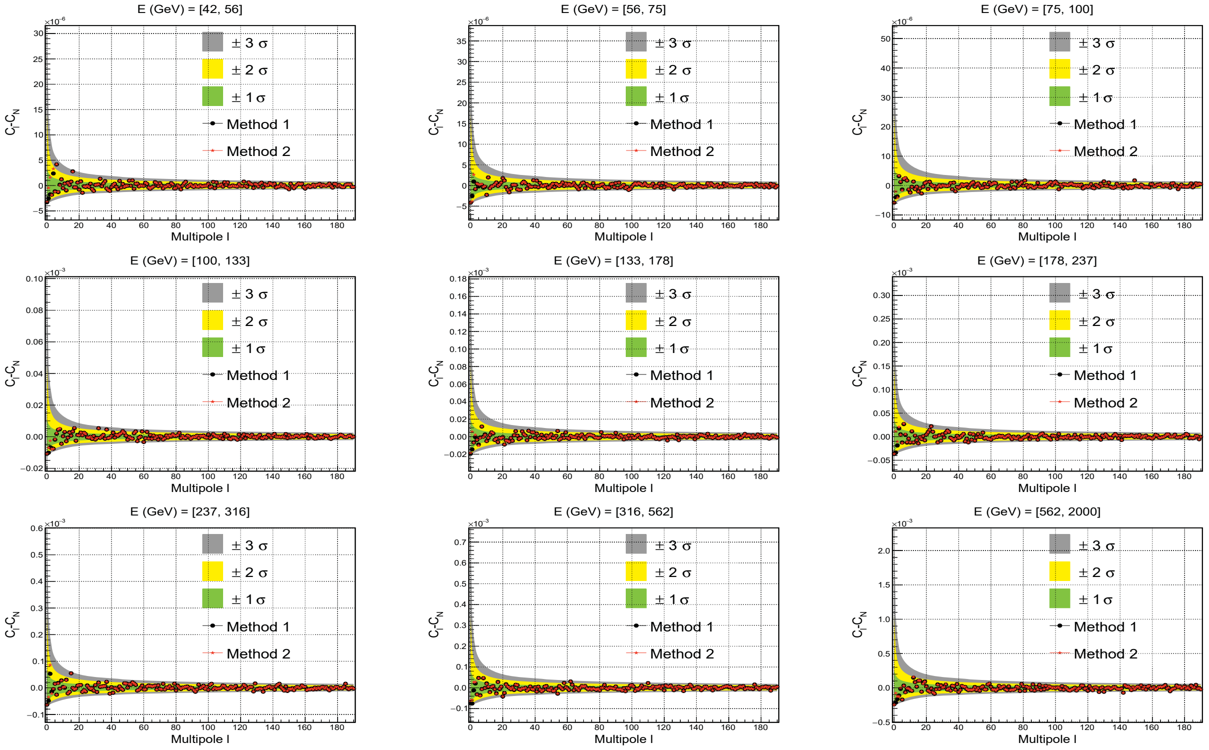


FIG. 16. Same as Fig. 15, but showing a wider range in multipole.

corresponding limit for $\hat{\delta}$ can be calculated from Eq. 7.

### Bayesian intervals

A Bayesian posterior probability can be used to calculate intervals that have a given probability of containing the true value of a parameter. From Eq. 8 the posterior probability $P(\hat{C}_1^{ani}|C_1, C_N)$ is given by:

$$P(\hat{C}_1^{ani}|C_1, C_N) \propto P(C_1|\hat{C}_1^{ani}, C_N)\pi(\hat{C}_1^{ani}) \quad (14)$$

where $\pi(\hat{C}_1^{ani})$ is the initial prior for the parameter $\hat{C}_1^{ani}$. The prior $\hat{C}_1^{ani}$ can be set according to Jeffreys' rule, and for this problem it is possible to show that

$$\pi(\hat{C}_1^{ani}) \propto \frac{1}{\hat{C}_1^{ani} + C_N} \quad (15)$$

The interval limit (called a Bayesian or credible interval) $[\hat{C}_{1,low}^{ani}, \hat{C}_{1,up}^{ani}]$ can be determined as the interval that contains a given fraction $1 - \alpha$ of the posterior probability, i.e.,

$$1 - \alpha = \int_{\hat{C}_{1,low}^{ani}}^{\hat{C}_{1,up}^{ani}} P(\hat{C}_1^{ani}|C_1, C_N) d\hat{C}_1^{ani} \quad (16)$$

The upper limit which contains a given fraction $1 - \alpha$ is calculated by setting $\hat{C}_{1,low}^{ani} = 0$, for example the upper limit which contains the fraction of 95% of the posterior probability is calculated from Eq. 16 setting $\alpha = 5\%$ and $\hat{C}_{1,low}^{ani} = 0$. Once the limit on $\hat{C}_{1,up}^{ani}$ is known, the corresponding limit for $\hat{\delta}$ can be calculated from Eq. 7.

## ACKNOWLEDGMENTS

The Fermi LAT Collaboration acknowledges generous ongoing support from a number of agencies and institutes that have supported both the development and the operation of the LAT as well as scientific data analysis. These include the National Aeronautics and Space Administration and the Department of Energy in the United States, the Commissariat à l'Energie Atomique and the Centre National de la Recherche Scientifique / Institut National de Physique Nucléaire et de Physique des Particules in France, the Agenzia Spaziale Italiana and the Istituto Nazionale di Fisica Nucleare in Italy, the Ministry of Education, Culture, Sports, Science and Technology (MEXT), High Energy Accelerator Research Organization (KEK) and Japan Aerospace Exploration Agency (JAXA) in Japan, and the K. A. Wallenberg Foundation, the Swedish Research Council and the Swedish National Space Board in Sweden. Additional support for science analysis during the operations phase

is gratefully acknowledged from the Istituto Nazionale di Astrofisica in Italy and the Centre National d'Études Spatiales in France.

The authors acknowledge the use of HEALPix `http://healpix.sourceforge.net` described in K.M. Gorski et al., 2005, Ap.J., 622, p.759. S. B. and S. G acknowledge support as a NASA Postdoctoral Program Fellow, USA. M.R. acknowledges funded by contract FIRB-2012-RBFR12PM1F from the Italian Ministry of Education, University and Research (MIUR).

* francesco.costanza@cern.ch

† mazziotta@ba.infn.it

[1] M. Ackermann *et al.* (Fermi-LAT Collaboration), Phys. Rev. **D82**, 092003 (2010), arXiv:1008.5119 [astro-ph.HE].

[2] S. S. Campbell, Mon. Not. Roy. Astron. Soc. **448**, 2854 (2015), arXiv:1411.4031 [astro-ph.CO].

[3] R. Iuppa and G. Di Sciascio, Astrophys. J. **766**, 96 (2013), arXiv:1301.1833 [astro-ph.IM].

[4] S. Abdollahi *et al.* (Fermi-LAT Collaboration), To be published (2017).

[5] E. Thébault *et al.*, Earth, Planets and Space **67**, 1 (2015).

[6] M. Aguilar *et al.* (AMS Collaboration), Phys. Rev. Lett. **114**, 171103 (2015).

[7] M. Aguilar *et al.* (AMS Collaboration), Phys. Rev. Lett. **113**, 121102 (2014).

[8] T. P. Li and Y. Q. Ma, Astrophys. J. **272**, 317 (1983).

[9] M. Fornasa *et al.*, Phys. Rev. **D94**, 123005 (2016), arXiv:1608.07289 [astro-ph.HE].
